# Supplementary material for: Benchmarking Early Agitation Prediction in Community-Dwelling People with Dementia Using Multimodal Sensors and Machine Learning
Source: arXiv:2506.06306 source file (2025-05-23)
Supplement: Supplementary file 1 [file additional-information.pdf]

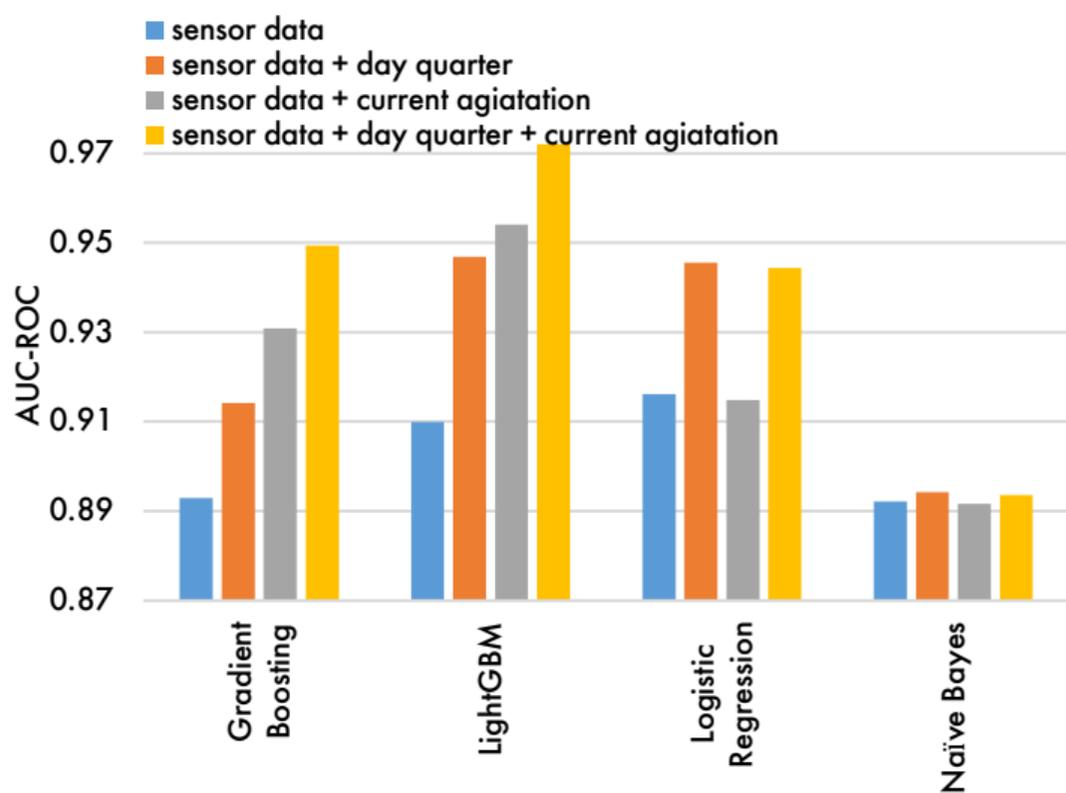

(a)

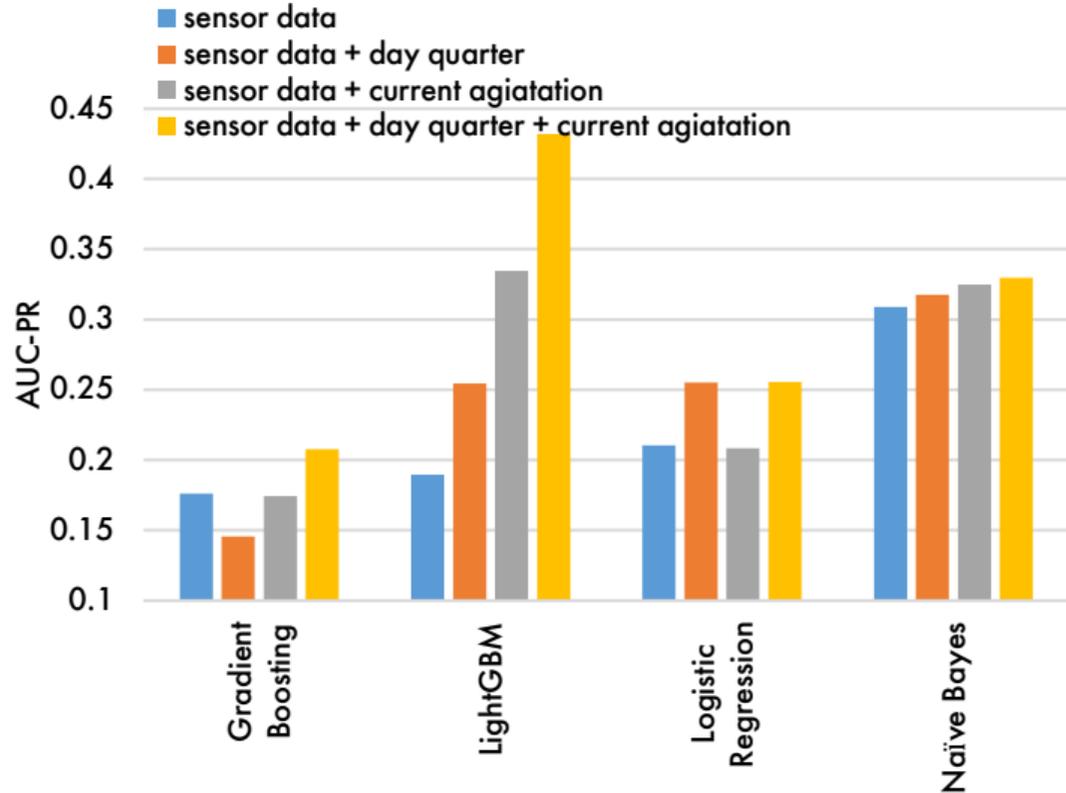

(b)

Figure 3. (a) AUC-ROC and (b) AUC-PR for agitation prediction framed as a binary classification problem using tabular sensor data under 5-fold cross-validation, following the incorporation of additional information: day quarter and current agitation status.
